# Supplementary material for: "Where Can I Park?" Understanding Human Perspectives and Scalably Detecting Disability Parking from Aerial Imagery
Source: arXiv:2509.25460 ancillary file (2025-09-29)
Supplement: Supplementary file 1 [file Design_Probes.pdf]

# Route Planning

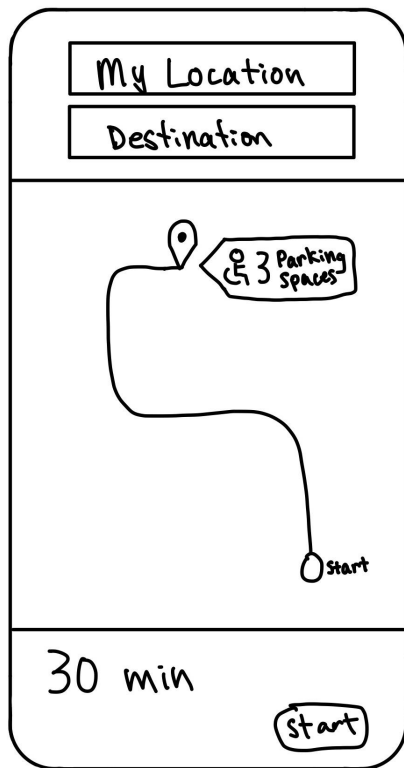

Parking count visible  
during route planning

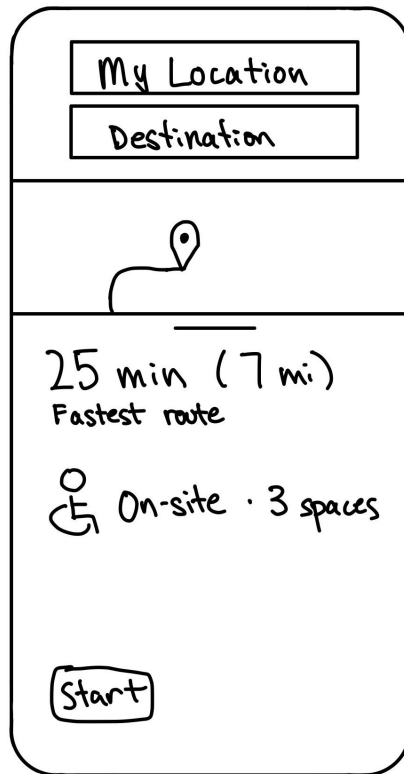

Parking count visible  
during route planning

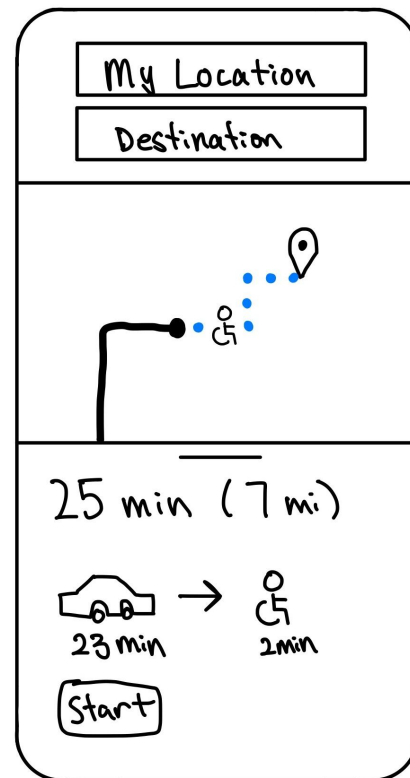

Path to entrance visible  
during route planning

# POI Investigation

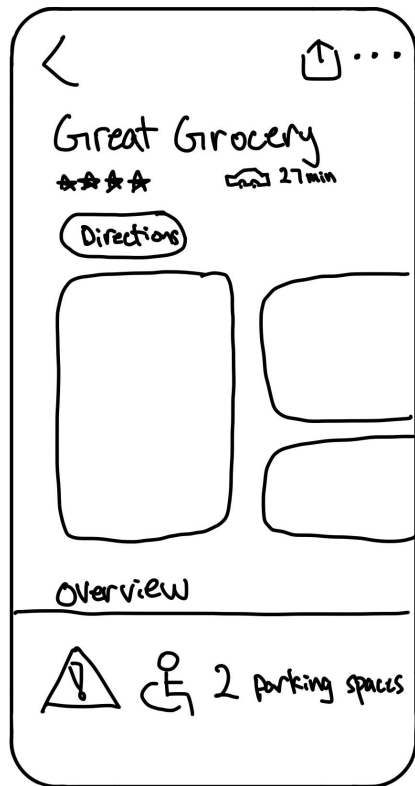

Parking space overview

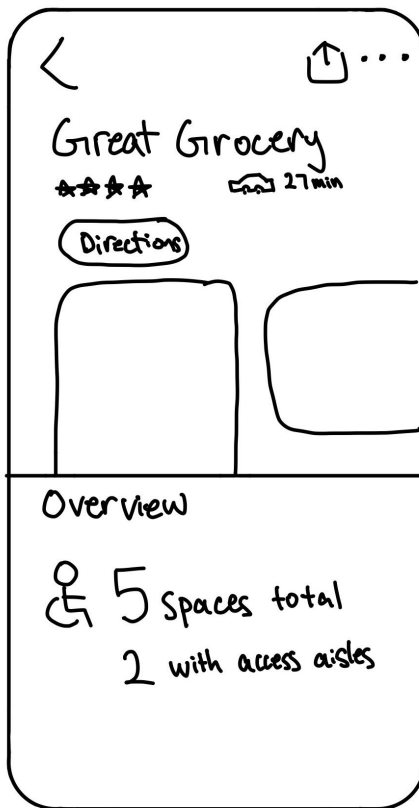

Parking space detailed overview

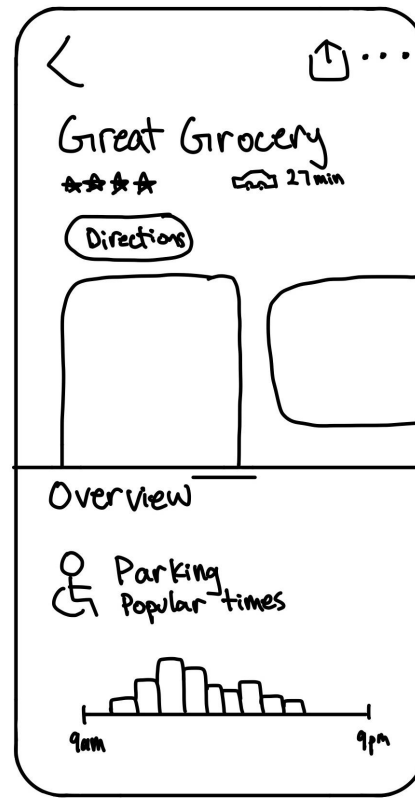

Parking space popular times

# In Situ Navigation

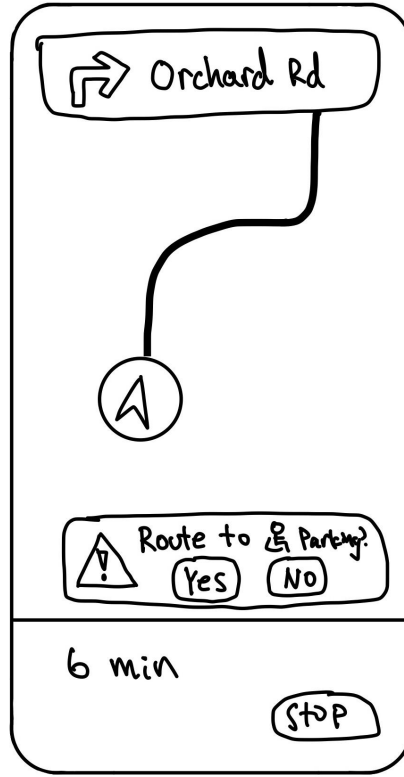

Parking routing popup

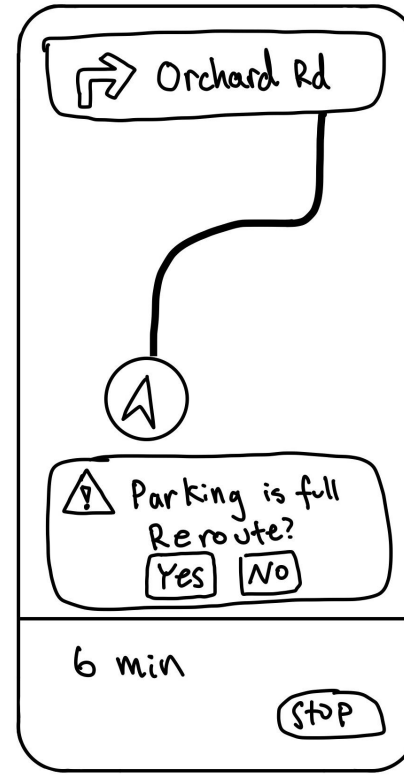

Parking full notification popup

# Out-of-car Experience

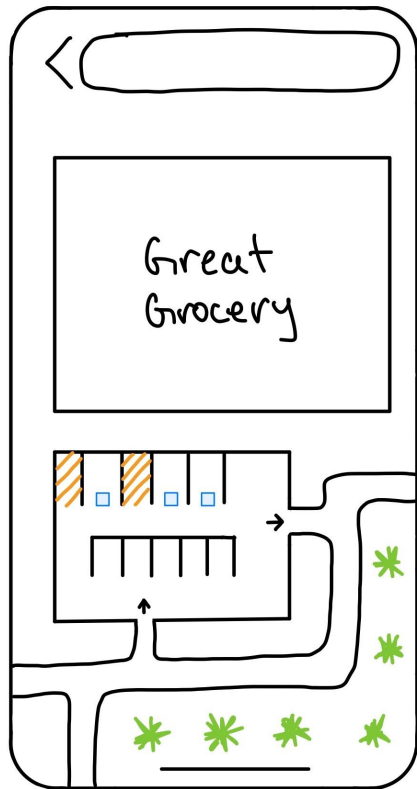

Detailed disability parking context

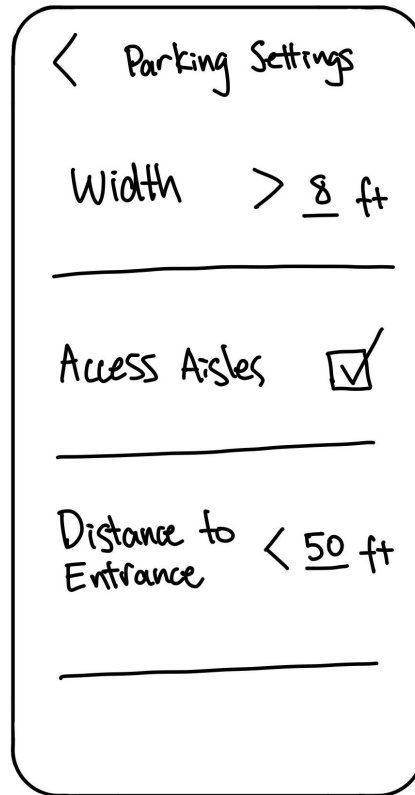

Route planning preferences

# Curbside

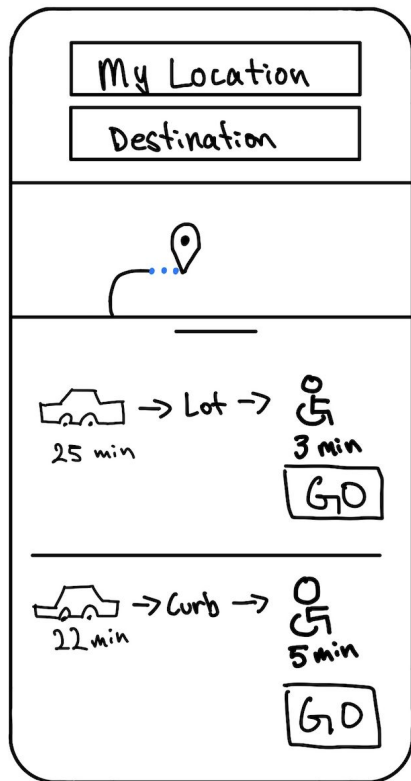

Routing with parking options

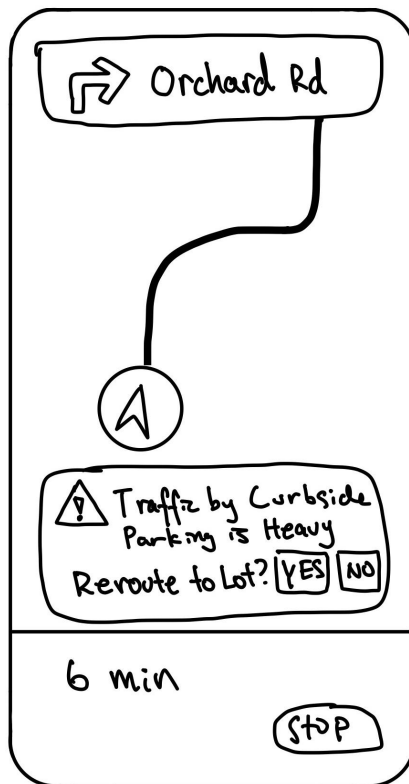

Reroute when lot parking conditions are poor

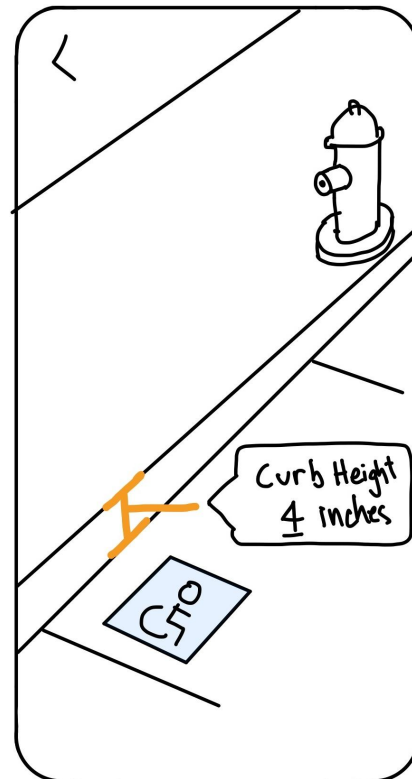

3D visual
