# Supplementary material for: "Where Can I Park?" Understanding Human Perspectives and Scalably Detecting Disability Parking from Aerial Imagery
Source: arXiv:2509.25460 ancillary file (2025-09-29)
Supplement: Supplementary file 2 [file Disability_Parking_Interview_Protocol__Clean_.pdf]

# Interview Protocol

## Part 1: Experiences with Parking and Transit (*10-15min*)

1. Can you **describe your disability**?
2. How does your **disability impact your ability** to move around both indoors and outdoors?
3. Tell me how you get around to places. [Trips to work, grocery stores, how often, with other people, etc.]
4. Tell me about how you plan to travel to an unfamiliar place—like a restaurant—for the first time.
5. How do you decide on what **mode of transportation** to take to a given destination?
6. Do you use any tools when planning or taking or taking a trip? Please describe them.
  - a. Would you use some tool that shows allocation, availability, or location of disability parking spots?
7. [If they don't drive most of the time or at all] What is your thought process on choosing not to drive?

## Part 2: Disability parking (*15-20 min*)

1. Do you **qualify for disability parking**? If so, for how long (have they qualified)? Do you or the person who drives you (if you don't drive) have a **disability parking placard**? Do you use **disability parking**?
2. What **challenges** have you faced when using disability parking?
  - a. Could you describe a specific instance where you faced a challenge? What did you do?

3. How much concern do you have over the availability [existence and capacity] of disability parking at your destination? Please explain.
4. What attributes do you think make a “good” parking space? Do you look for anything in particular when you’re parking somewhere? [If stuck, can ask if they have a favorite/least favorite parking space somewhere they frequent, and why]
5. Do you have any concerns about the state of disability parking where you live?
  - a. Is there enough?
  - b. Is it placed well?
  - c. Is there enough space for your needs?
  - d. How about disability parking violations (parking in a disability parking space without a placard)? Does this impact you significantly?
6. Do you **prefer streetside parking** or **parking** in a **lot**? Why?
7. Do you ever decide not to drive somewhere specifically because of the parking at the destination? Why? Describe your thought process.

## Part 3: Technology and Design (10-15 min)

In this section, I'm going to mention existing technologies, and I'd like you to respond if you use them/don't use them and when/why.

1. Routing tools (Google Maps, Apple Maps, OpenStreetMap)
2. Taxis/ridesharing apps (like Uber/Lyft etc.)
3. Autonomous vehicles. E.g., Tesla full self driving.

Now, I'd like to take the rest of the time to brainstorm new potential technologies related to disability parking.

1. [Show probes in Powerpoint] Here are some mockups that we've created.
  - a. Would something like this be useful?
  - b. Do you have any suggestions or ideas regarding these mockups? There are no wrong answers.
2. Thinking beyond these examples, what other features might be useful for you? There are no limitations.

## Payment

1. We can provide compensation in the form of a Tango gift card (a gift card service that lets you buy gift cards to other services) or an Amazon gift card. Do you have a preference?
2. We will send a followup email asking for some information in order for us to provide you with the gift card. Unfortunately, after that, it may take some time before everything is processed (maybe up to a month or more). Thank you for your patience.
