# Supplementary material for: "Where Can I Park?" Understanding Human Perspectives and Scalably Detecting Disability Parking from Aerial Imagery
Source: arXiv:2509.25460 ancillary file (2025-09-29)
Supplement: Supplementary file 3 [file screener_pdf.pdf]

## Default Question Block

We want to understand how people use disability parking, and what we can do to improve it. Help us by providing your insight!

We are looking for people over 18 years of age, who are eligible for disability parking and live in the US. Please fill out this screener if you're interested in participating. If you meet the criteria, we may reach out to schedule an around one hour interview over the remote platform Zoom. Upon completion of the interview we will compensate you \$25/hr.

For questions, reach out to

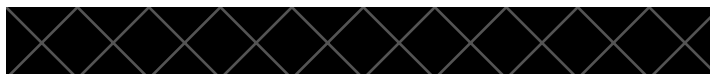

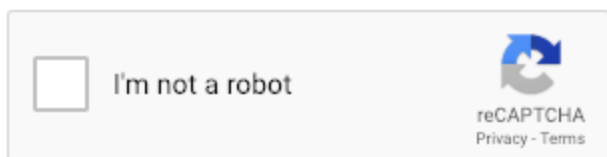

## Block 1

What is your name?

How old are you?

- ☐ Under 18 years
- ☐ 18 to 24 years
- ☐ 25 to 34 years
- ☐ 35 to 44 years
- ☐ 45 to 64 years
- ☐ 65 to 84 years
- ☐ 85 to 99 years
- ☐ 100 years and over

What is your email?

Which of the following best describes where you live?

- ☐ Rural (less than 2,500 people)
- ☐ Town (2,500 to 50,000 people)
- ☐ City (more than 50,000 people)

Do you identify as having a disability? If so, what is your

disability?

Are you eligible to use disability parking?

- ☐ Yes
- ☐ No
- ☐ I don't know

How long have you been eligible to use disability parking?

How often do you travel outside the home during a typical week?

Please include both commute and personal trips

- ☐ Once a week or less
- ☐ 2 to 4 times
- ☐ More than 4 times

Powered by Qualtrics
